# Supplementary material for: Non-coalescence of sessile drops from different but miscible liquids: Hydrodynamic analysis of the twin drop contour as self stabilizing, traveling wave
Source: arXiv:1206.3699 source file (2012-06-16)
Supplement: Supplementary file 1 [file Supplemental.pdf]

## Mechanistic description of non-coalescence

To understand non-coalescence we have to understand first, what drives the coalescence of sessile drops in general. Then we have to analyze what is different in our case and suppresses the “usual” coalescence mechanisms. We even have to be more specific. Our experiments show that right after contact the drops start to coalesce. But after a short time the process towards coalescence somehow stops for some time (actually it can stop for a very long time compared to the initial transient process until, eventually the drops resume a coalescence process and fuse quite rapidly into a single drop). During this time of temporary stationary non-coalescence liquid continuously flows from one drop into the other through the thin neck that connects the two drops. The temporary state of non-coalescence is a twin-drop configuration with a thin neck in between.

The general reason for drop coalescence is basic (interfacial) physics: As soon as two sessile drops get in contact, they will proceed to coalesce because this minimizes the system surface respectively surface energy. The "mechanism" is capillary. More specifically it is the capillary pressure, which is parametrized by the surface curvature. An analysis of the coalescence behavior for drops with identical (I.) respectively different (II.) liquids yields the following:

I.) Identical liquids.

With identical liquids (i.e., identical surface tensions), the capillary pressure that drives coalescence is the pressure difference between the drop volumes (positive, comparatively small curvature) and the neck (negative, comnparatively large curvature). Compared to the pressure difference between neck and drop, the pressure difference between the two drops is negligible because we focus here on the case with a pronounced neck between two drops of macroscopic size (i.e., millimeter-sized or larger, but smaller than the capillary length). This means, to a first approximation, different absolute (and relative) drop sizes have only a minor quantitative impact on the Laplace pressure and thus on the coalescence behavior. The neck curvature mostly determines the strength of the pressure and the flow is always from both drop volumes TOWARDS the neck, which per definition is the region of the lowest pressure (largest curvature). With identical liquids there is no other mechanism causing a flow. Hence there is no flow component away from the neck and nothing stops the two drops from fusing into a single one.

II.) Different liquids.

With different liquids there are two contributions that cause flow:

IIa) Capillary contribution.

If the drops consist of different, but completely miscible liquids (with different surface tensions), regarding capillarity the situation is qualitatively the same as with identical liquids. The flow originating from capillarity will be dominated by the neck curvature with (minor) modifications due to different drop sizes and different surface tensions. All the flow *driven by capillary* is directed only TOWARDS the neck.

IIb) Marangoni contribution.

With different liquids, surface tension gradients are an additional source of flow (Marangoni). Local surface tension gradients will (temporarily) appear after drops with different liquids respectively surface tensions get in contact. It turns out, that in the case of temporarily stationary non-coalescence a temporarily stationary local gradient establishes near the neck, on the drop with the higher surface tension. Surface tension gradients can only appear on this drop because the Marangoni flow is always directed towards the location with the higher surface tension side of the gradient. There is never a Marangoni

flow into the drop with lower surface tension, only into the drop with higher surface tension. The asymmetry respectively direction of the Marangoni flow is important. Capillary only induces flows from both drop volumes TOWARDS THE NECK whereas Marangoni adds an asymmetrical flow component, a flow component OUT OF THE NECK REGION into the drop with the higher surface tension. This flow component empties the neck i. e., it opposes filling the neck (coalescence) driven by the capillary flow component (in our theoretical derivation this is formally taken into account by the continuity equation, which is *embedded* in the film equation to obtain the temporal derivative of the local film height, $\partial_t h$ (see below)). Thus Marangoni works against coalescence. The result can be a temporarily stationary state of non-coalescence. The movement of the stationary non-coalescing twin drop configuration over the substrate results from the asymmetric net flow between the drops towards the drop with the higher surface tension.

To explain the temporary stationarity of the twin drop configuration is not straightforward. Supposedly the different flow components temporarily just compensate each other such that the neck is stabilized. Obviously their strengths just scale antagonistically with neck height. It is also anything from obvious that the diffusive-advective dilution leads a stationary, stabilizing surface tension gradient. Nevertheless, the stabilization mechanisms appear to be rather robust because a stationary state of non-coalescence is observed for a wide range of parameter values. Our theoretical approach is based on these ideas and observations. The focus of the theoretical description is the stationary state. The transition states i.e., the beginning of coalescence right after drop contact as well as the final drop coalescence are not in the focus of our analysis although certain dynamic properties, such as the lifetime of the non-coalescence state can be derived/estimated from the stationary analysis.

The key to a theoretical description of the stationary state is its apprehension as a stationary twin drop profile moving at constant speed over the substrate. Therefore it is described by a stationary solution of the time-dependent thin film equation

$$\partial_t h = -\frac{1}{\eta}\partial_x \left[\gamma \frac{h^3}{3}\partial_x^3 h + \frac{h^2}{2}\partial_x \gamma\right] . \tag{1}$$

In our case this means we have to find a stationary contour of a liquid volume that is constantly moving over a substrate i. e., a solution of Eq. 1 of the manuscript (which is the time-dependent thin film equation with $\partial_t h$ replaced by $-v_N \partial_x h$ and integrated once). This is not straighforward because of the localized $\partial_x \gamma$. Therefore we first look for a (non-trivial) solution of Eq. 1 of the manuscript for the case without surface tension gradient (Eq. 1 without the Marangoni term).

There exists indeed a non-trivial stationary solution with a moving liquid (Eqs. 6 and 7). However, the corresponding profile describes only a single drop that is connected to an infinite liquid volume. This is not what we observe. If we take into account (by asymptodic matching) however a local Marangoni flow, which we describe based on the experimental findings, then we find a contour that matches the stationary twin-drop configuration. Simply speaking, the Marangoni flow shapes the infinite volume into a second drop. With proper boundary conditions we obtain the twin drop moving contour with properties that match quite well the experimental findings.

# Estimating the Impact of the Surface Tension Gradient

In Eqs. 10 and 11 of the main letter, the analytical profile (which is not subject to surface tension gradients) is used to approximate the "real" integrand. At first sight this is wrong since the gradient influences the profile (see Fig. 1 A: without gradient, the profile diverges after the neck; with gradient, a second drop is found). Within experimental parameter ranges however, the surface tension gradient is localized close to the neck (see Fig. 1 B). This, together with the fact that *in both cases* the profile height grows fast after the gradient, justifies the approximation: The integrand contains only negative powers of $h$. Fig. 1 shows the exact and approximated integrands; the value of the integrals are given by the areas under the curves (shaded). Within experimental parameters the approximation is very good (relative errors $< 20\,\%$).

The integral to estimate the asymptotic curvature can be evaluated analytically by substituting $y = x/(h_N Bo)$ and $k = Bo\,[3/2 Ca]^{1/3}\sqrt{-s_2}$, and the development of $h_{\gamma'=0}(x)$ in powers of $x$ up to second order:

$$\begin{aligned}\frac{3}{2\gamma_2}\int_0^\infty \frac{\gamma'}{h_{\gamma'=0}}dx &\approx \frac{3\Delta\gamma}{4\sqrt{2\pi}\gamma_2 h_N}\int_0^\infty \frac{e^{-1/8y}}{y^{3/2}(1+k^2y^2)}dy \\ &= \frac{3\Delta\gamma}{2\gamma_2\,h_N}\left\{ 1+\frac{1}{4}\sqrt{\pi\,k}\left\{ \left[1-2\,\mathrm{FrC}\left(1/2\sqrt{k/\pi}\right)\right]\,\sin\left(k/8\right) \right.\right. \\ &\qquad \left.\left. -\left[1-2\,\mathrm{FrS}\left(1/2\sqrt{k/\pi}\right)\right]\,\cos\left(k/8\right)\right\}\right\}. \end{aligned} \tag{2}$$

To a very good approximation, sine, cosine and the Fresnel integrals can developed in powers of $k$:

$$\frac{3}{2\gamma_2}\int_0^\infty \frac{\gamma'}{h_{\gamma'=0}}dx \approx \frac{3\Delta\gamma}{2\gamma_2 h_N}\left\{1+\sqrt{\pi\,k}/4+k(\pi+k/3)/16\right\} \tag{3}$$

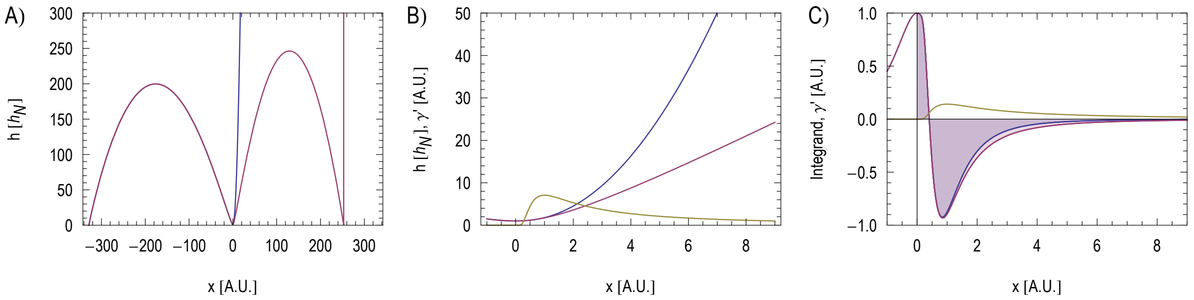


**Figure 1:** *A) Typical non-coalescing drop profiles: analytic solution for a single drop (blue) and numerical solution including surface tension gradient (red). B) zoom to the neck region, together with the surface tension gradient (yellow). C) Integrand used to estimate impact of gradient: exact numerical solution (red) compared to analytic estimate (blue). Shaded areas represent the integral.*

## The influence of shear-induced dispersion: Taylor-Aris correction

The effective diffusion coefficient resulting from the Taylor-Aris correction is typically described by:

$$D_{eff} = D(1 + (1/a)Bo^2), \tag{4}$$

with $D$ as diffusion coefficient without flow and $a$ as factor reflecting the flow geometry (with $a >> 1$, typically between 10 and 200). In our case, with typically $D = 10^{-10}m/s$, $h_{neck} = 10^{-6}m$ and $v = 10^{-3}m/s$, $Bo^2 = 100$, $D_{eff}$ might indeed differ significantly from $D$.

In a *stationary* state, taking the Taylor-Aris dispersion into account, means in our case (to a first approximation) replacing the "normal" Diffusion coefficient by an *effective* (i.e., larger) diffusion coefficient. Qualitatively, this does not change our theoretical approach. Even quantitatively the modifications are not very pronounced if we just vary $D$, as can bee seen from Fig. 5 in the manuscript.

## Estimation of the lifetime (dwell-time) of the state of non-coalescence

The dwell time $t_d$ on the non-coalescing state may be estimated from the model results: The rate of change for the surface tension difference $d\,\widetilde{\Delta\gamma}/dt \approx \widetilde{\Delta\gamma} h_N v_N / A_2$ can be integrated numerically between the initial $\widetilde{\Delta\gamma}_i$ and the (experimental) critical $\widetilde{\Delta\gamma}_c$. For the largest experimental surface tension differences in Fig. [2] of the manuscript, the predicted dwell times $t_d \approx 0.6\,\mathrm{s}, 2.1\,\mathrm{s}, 6.5\,\mathrm{s}$ for $\eta \approx 1.7\,\mathrm{cP}, 4.6\,\mathrm{cP}, 15\,\mathrm{cP}$ respectively, match well with the experimental values ($t_d \approx (0.6 \pm 0.2)\,\mathrm{s}, (1.6 \pm 0.5)\,\mathrm{s}, (8 \pm 2)\,\mathrm{s}$; the errors reflect the reproducibility of individual experiments).
